# Supplementary material for: Demystifying CXL Memory with Genuine CXL-Ready Systems and Devices
Source: arXiv:2303.15375 source file (2023-10-05)
Supplement: Supplementary file 1 [file 11-appendix.tex]

%\clearpage
\appendix
\section{Artifact Appendix}

\subsection{Abstract}
This appendix explains how to reproduce the results presented in this paper, which is based on an evaluation platform described in Table~\ref{table:config-table}.
In the following sections, we provide guidelines to access, build, and setup the environments for individual (micro)benchmarks evaluated in this work.
We also provide a set of scripts that automatically collect the results after running experiments.
The artifact is available publicly through an archived repository.

\subsection{Artifact check-list}
{\small
\begin{itemize}
  \item {\bf Program: } 
  \begin{itemize}
  \item Intel MLC (Memory Latency Checker) v3.10~\cite{mlc}: \figref{fig:seq_latency}, \ref{fig:seq_bandwidth}.
  \item \arch: \figref{fig:seq_latency}, \ref{fig:seq_bandwidth}.
  \item \texttt{YCSB} (Yahoo! Cloud Serving Benchmark)~\cite{socc10:ycsb}: \figref{fig:app:latency}, \ref{fig:ycsb_max_qps}, \ref{fig:tune-improvement}. 
  \item \texttt{Redis}~\cite{redis}: \figref{fig:app:latency}, \ref{fig:ycsb_max_qps}, \ref{fig:tune-improvement}.
  \item \texttt{DSB} (DeathStarBench)~\cite{deathstartbench}: \figref{fig:app:latency}.
  \item \texttt{FIO} (Flexible I/O Tester)~\cite{GitHubax76:online}: \figref{fig:app:latency:fio:log-scale}.
  \item \texttt{MERCI}~\cite{asplos21lee}: \figref{fig:ycsb_max_qps}, \ref{fig:correlation}, \ref{fig:linear-model-throughput}.
  \item \texttt{SPEC CPU2017}~\cite{SPECCPU70:online}: \figref{fig:linear-model-throughput}, \ref{fig:tune-improvement}.
  \item \policy: \figref{fig:linear-model-throughput}, \ref{fig:tune-improvement}.
  \end{itemize}
  \item {\bf Compilation: } GCC-11.4.0 (\arch, FIO, SPEC2017, MERCI), Maven 3 (YCSB). For the other benchmarks, please refer to their repository for proper environemnet setup.
  \item {\bf Binary: } Intel MLC v3.10, Redis, DeathStarBench.
  \item {\bf OS environment: } Ubuntu 22.04.2 LTS with different kernel versions and patches.
  \begin{itemize}
      \item \textbf{TPP-related tests:} Linux kernel v5.13 with TPP patch ~\cite{tpp-patch}.
      \item \textbf{\policy, memory interleaving tests:} Linux kernel v5.19 with m-n memory interleave patch ~\cite{mn_il_patch}.  
      \item \textbf{Else:} Linux kernel v6.2.
  \end{itemize}
  \item {\bf Hardware: } An evaluation platform with dual-socket Intel Xeon 6430 CPUs, 8-channel DDR5-4800 modules for socket 0, 1-channel DDR5-4800 module for socket 0, and three CXL devices (Table~\ref{table:config-table}).
  \item {\bf Run-time state: } Fixed CPU frequency (2.1~GHz), Turbo Boost/Hyper-Threading off.
  \item {\bf Metrics: } The artifact reports memory access latency (ns), memory bandwidth (GB/s), or application throughput (query per second for Redis, inference per second for DLRM). 
  \item {\bf Output: }\texttt{.txt} files including collected metrics corresponding to individual experiments.
  \item {\bf Experiments reproduced: } \figref{fig:seq_latency}, \ref{fig:seq_bandwidth}, \ref{fig:app:latency}, \ref{fig:app:latency:fio:log-scale}, \ref{fig:ycsb_max_qps}, \ref{fig:tune-improvement}.
  \item {\bf How much disk space required (approximately)?: } 20~GB storage for DeathStarBench docker images, 50~GB storage for FIO, 5~GB for MERCI dataset.
  \item {\bf How much time is needed to prepare workflow (approximately)?: } More than 3 hours.
  \item {\bf How much time is needed to complete experiments (approximately)?: } More than 48 hours.
  \item {\bf Publicly available?: } Yes. 
  \item {\bf Code licenses (if publicly available)?: } GPL v2.0.
  \item {\bf Archived: } \url{https://zenodo.org/record/8332543}
\end{itemize}
}

\subsection{Description}

\subsubsection{How to access}
Our own microbenchmark (\arch) and proposed page allocation software (\policy) are archived at Github and Zenodo. The other (micro)beanchmarks (except for SPEC CPU2017) are open-sourced that are publicly available at:
\begin{itemize}
    \item Intel MLC v3.10: \url{https://www.intel.com/content/www/us/en/download/736633/763324/intel-memory-latency-checker-intel-mlc.html}
    \item \texttt{YCSB}: \url{https://github.com/brianfrankcooper/YCSB}
    \item \texttt{Redis}: \url{https://github.com/redis/redis}
    \item \texttt{DSB}: \url{https://github.com/delimitrou/DeathStarBench}
    \item \texttt{FIO}: \url{https://github.com/axboe/fio}
    \item \texttt{MERCI}: \url{https://github.com/SNU-ARC/MERCI}
    %\item mn interleave kernel patch: \url{https://lore.kernel.org/linux-mm/20220607171949.85796-1-hannes@cmpxchg.org/} 
\end{itemize}

%Since CXL devices and supported CPUs are hard to order, we can provide access to these hardware systems for AE purposes, as they are currently setup in the FAST Lab of UIUC-ECE. These systems can be accessed via UIUC VPN (software environment/libraries/benchmarks setup already). Please contact us for setting up connection to our servers. 

\subsubsection{Hardware dependencies}
We conduct evaluations on an Intel SPR platform equipped with three types of CXL memory devices, as described in Table~\ref{table:config-table}. Sub-NUMA clustering mode (SNC) is disabled for Intel MLC and \texttt{memo} and enabled (\ie, SNC-4) for the later experiments. For a fair comparison with the local CXL memory devices each of which uses a single PCIe link, we limit the remote DDR5 memory to use only a single DRAM channel, as follows:

\begin{lstlisting}
- Socket 0 (Local)
    - DIMM 0 <Inserted>
    - DIMM 1 <Inserted>
    ...
    - DIMM 7 <Inserted>
- Socket 1 (Remote)
    - DIMM 0 <Inserted>
    - DIMM 1 <Not used>
    ...
    - DIMM 7 <Not used>
\end{lstlisting}

\subsubsection{Software dependencies}
Our testbed runs Ubuntu 22.04.3 LTS with kernel version 6.2. Most native installation of Ubuntu does not come with \texttt{libnuma}, which is used in \arch for allocating memory on a specific NUMA node. The following command will install \texttt{libnuma} on Ubuntu.

\begin{lstlisting}
$ sudo apt install libnuma-dev
\end{lstlisting}

\noindent Additionally, we use \texttt{cpupower} to fix the CPU frequency to 2.1~GHz in all experiments. The following command will install Linux tools including \texttt{cpupower} on Ubuntu.
\begin{lstlisting}
$ sudo apt install linux-tools-$(uname -r)
\end{lstlisting}

%For the SPEC benchmarks, UIUC has SPEC benchmarks licensed under Prof. Saugata Ghose. Our machine has SPEC benchmark installed. 

\noindent For the rest of the benchmarks, please follow the guidelines in GitHub pages to setup the corresponding environments. %These environment, including the one for \policy, has been setup on our machine.

\subsection{Installation}
To install \arch or \policy,  we first need to clone the source code:
\begin{lstlisting}
$ git clone https://github.com/ece-fast-lab/cxl_type3_tests
\end{lstlisting}
% \begin{lstlisting}[escapeinside={(*@}{@*)}]
% $ git clone (*@\href{https://github.com/ece-fast-lab/cxl_type3_tests}{https://github.com/ece-fast-lab/cxl\_type3\_tests}@*)
% \end{lstlisting}

\noindent Then, go to the source code directory:
\begin{lstlisting}
$ cd memo_ae/src
\end{lstlisting}

\noindent Finally, build the executable binary from the source code:
\begin{lstlisting}
$ make
\end{lstlisting}

\noindent To test \policy, please go to the source code directory for \policy:

\begin{lstlisting}
$ cd caption_ae/src
\end{lstlisting}

%%%%%%%%%%%%%%%%%%%%%%%%%%%%%%%%%%%%%%%%%%%%%%%%%%%%%%%%%%%%%%%%%%%%%
\subsection{Experiment workflow}
\label{sec:workflow}

We provide guidelines for BIOS configuration as well as automated scripts for all evaluated workflows. Within these scripts, the common operation goes as follows:
\begin{lstlisting}
$ # set software / hardware environment
$ # run application in loops
$ # unset the environment
\end{lstlisting}

\noindent In most cases, BIOS configuration involves enabling and disabling Sub-NUMA clustering (SNC) and hyperthreading. In the software level, Setting and un-setting the environment involves locking/unlocking the CPU frequency, and creating cgroup directories for fine-grain control over cpu and memory resources. Detailed experiment steps for each experiment (regarding Figure~\texttt{X}) is available at the \texttt{config\_figure\_X.md} file in the folders of the repository.

\begin{comment}
\input{ae-appendix/05-1-eval_memo}
\input{ae-appendix/05-2-eval_ycsb_redis}
\input{ae-appendix/05-3-eval_dsb}
\input{ae-appendix/05-4-eval_fio}
\input{ae-appendix/05-5-eval_dlrm}
\input{ae-appendix/05-6-eval_caption}
\end{comment}

\subsection{Evaluation and expected results}

After running each experiment (\S\ref{sec:workflow}), the result data (memory access latency and bandwidth, application throughput, \textit{etc.}) can be automatically collected using a provided script corresponding to each figure. For more detailed instructions, please refer to each \texttt{run\_figure\_X.md} file in the repository.

\subsection{Experiment customization}
To run DeathStarBench with the proper NUMA node in \figref{fig:dsb_compose}, \ref{fig:dsb_read_user}, and \ref{fig:dsb_mixed}, we modify the following docker images to pin their CPU and memory to the desired NUMA node.
\begin{itemize}
    \item MongoDB: Change entrypoint.sh
    \item Redis: Install numactl
    \item Memcached: Install numactl
\end{itemize}

\noindent For Redis and Memcached, the \texttt{numactl} command is embedded in the docker-compose file, whereas MongoDB requires manual changes to the \texttt{entrypoint.sh} within the docker image. Please refer to the \texttt{setup\_docker.md} in the repository for the detailed steps in modifying the docker images.
